# Supplementary material for: Neural Appearance Modeling From Single Images
Source: arXiv:2406.18593 source file (2024-06-08)
Supplement: Supplementary file 1 [file n_A_ggx_appendix.tex]

\section*{Appendix A}
\label{ggx_discussion}
\addcontentsline{toc}{section}{Appendix}
\subsection{Microfacet GGX BRDF}
A microfacet model describes how light interacts with a rough surface by representing a point as a collection of un-observable, tiny, mirror-like facets. Each micro-facet has its own orientation, and the appearance of a surface point is determined by the distribution of the orientations of its micro-facets, which are often modeled by a \textbf{normal distribution function (NDF)}. The NDF takes a normal direction returns the probability density of the normal direction (projected onto the rough micro-facet surface). For any incident light direction, l, and outgoing view direction, v, only micro-facets with orientation equal to the half-way direction, $h = (l + v) / ||(l + v)||$, will reflect light from l to v.

The Trowbridge-Reitz GGX micro-facet model's NDF, proposed by Trowbridge and Reitz \cite{trowbridge1975average} and re-discovered by Walter et al. \cite{walter2007microfacet}, uses the following NDF:

\[ D(h) = \frac{\alpha^2}{\pi \left( (\cos(\theta_h)^2) \left( \alpha^2 - 1 \right) + 1 \right)^2} \]
where \( \theta_h \) is the angle between the normal of the surface \( n \) and the micro-facet normal \( h \), and \( \alpha \) represents the standard deviation of the surface slope distribution. \( \alpha \) controls the spread of the micro-facet normals; smaller values of lead to a distribution concentrated at the macro-normal (smooth surfaces), while larger values produce a broader distribution (rough surfaces).

For a given light and view direction, a \textbf{shadow-masking term} is used to approximate the fraction of micro-facets with orientation equal to h that are actually visible to both directions. The Smith approximation \cite{smith1967geometrical} for the shadow-masking term of GGX is: 
\[ G_1(i, h) = \frac{(i \cdot h)}{(i \cdot h) * (1.0 - (0.5*\alpha)) + 0.5*\alpha} \]

\[ G(v, l, h) = G_1(v, h)\ G_1(l, h)\]
where v is the outgoing view direction, l is the incident light direction, h is the half-way direction; and $(x \cdot y )$ is the dot product of x and y.

Finally, the \textbf{Fresnel term} approximates the ratio of reflected light to incident light, for visible micro-facets with orientation h. The remaining light is refracted (or diffusely scattered), not mirror-reflected. The approximated Fresnel term using Schlick's approximation \cite{schlick1994inexpensive} is: 
\[ F(v, h) = F_0 + (1 - F_0)(1 - \cos(v \cdot h))^5 \]
where \( F_0 \) represents the specular reflectance at normal incidence.

These terms can then be combined to form the complete GGX BRDF:
\[ f_{\text{GGX}}(v, l, h) = \frac{D(h)F(v, h)G(v, l, h)}{4(h \cdot v)(h \cdot l)} \] 
\\
In practice, the the GGX BRDF is augmented with a \textbf{diffuse term} accommodating equal light scatter in all directions. The diffuse term is often represented by a Lambertian reflectance model; where reflected radiance is proportional to the cosine of the angle between the incident light and the macro-surface normal (not a 'mirror-like' micro-facet normal).

\subsection{GGX SVBRDF Maps}
In practice, the GGX BRDF can be extended to an SVBRDF, which allows the reflectance properties to vary across a surface. An SVBRDF is typically implemented using various texture maps that store different material properties at each pixel (point) on the surface. For the GGX model, these maps are:

\textbf{The Diffuse Map} represents the base color of the material, which is the color of the light scattered in all directions.

\textbf{Specular Map} determines the color and intensity of the specular, mirror-like reflections.

\textbf{The Normal Map} provides perturbations to the spatially-varying surface normals to simulate surface perturbations. Each pixel encodes a direction, not a color.

\textbf{Roughness Map} captures the roughness parameter \( \alpha \) of the GGX model, which affects the distribution of micro-facet orientations and therefore the spread of the specular highlights. Typically each pixel encodes $\sqrt{\alpha}$ with values in [0, 1].
